# Supplementary material for: Absence of altermagnetic spin splitting character in rutile oxide RuO$_2$
Source: arXiv:2409.13504 source file (2024-11-08)
Supplement: Supplementary file 1 [file Supplementary.pdf]

# Supplementary information for

# "Absence of altermagnetic spin splitting character in rutile oxide $RuO_2$"


Jiayu Liu,[1,2,3,*] Jie Zhan,[4,5,*] Tongrui Li,[6,*] Jishan Liu,[2,7,†] Shufan Cheng,[8] Yuming Shi,[1,3] Liwei Deng,[1,3] Meng Zhang,[9] Chihao Li,[10] Jianyang Ding,[1,3] Qi Jiang,[11] Mao Ye,[2,7] Zhengtai Liu,[2,7] Zhicheng Jiang,[6] Siyu Wang,[6] Qian Li,[6] Yanwu Xie,[9] Yilin Wang,[12,13] Shan Qiao,[7,‡] Jinsheng Wen,[8,14,§] Yan Sun,[4,5,¶] and Dawei Shen[6,**]

[1]*Shanghai Institute of Microsystem and Information Technology, Chinese Academy of Sciences, Shanghai 200050, China*

[2]*Shanghai Synchrotron Radiation Facility, Shanghai Advanced Research Institute, Chinese Academy of Sciences, Shanghai 201210, China*

[3]*University of Chinese Academy of Sciences, Beijing 100049, China*

[4]*School of Materials Science and Engineering, University of Science and Technology of China, Shenyang 110016, China*

[5]*Shenyang National Laboratory for Materials Science, Institute of Metal Research, Chinese Academy of Sciences, Shenyang 110016, China*

[6]*National Synchrotron Radiation Laboratory and School of Nuclear Science and Technology, University of Science and Technology of China, Hefei 230026, China*

[7]*National Key Laboratory of Materials for Integrated Circuits, Shanghai Institute of Microsystem and Information Technology, Chinese Academy of Sciences, Shanghai 200050, China*

[8]*National Laboratory of Solid State Microstructures and Department of Physics, Nanjing University, Nanjing 210093, China*

[9]*School of Physics, Zhejiang University, Hangzhou 310027, China*

[10]*Laboratory of Advanced Materials, State Key Laboratory of Surface Physics, and Department of Physics, Fudan University, Shanghai 200438, China*

[11]*Center for Transformative Science, ShanghaiTech University, Shanghai 201210, China*

[12]*School of Emerging Technology, University of Science and Technology of China, Hefei 230026, China*

[13]*Hefei National Laboratory, University of Science and Technology of China, Hefei 230088, China*

[14]*Collaborative Innovation Center of Advanced Microstructures, Nanjing University, Nanjing 210093, China*

[*] Equal contributions
[†] Equal contributions; liujs@sari.ac.cn
[‡] qiaoshan@mail.sim.ac.cn
[§] jwen@nju.edu.cn
[¶] sunyan@imr.ac.cn
[**] dwshen@ustc.edu.cn

## Methods

### Synthesis of single-crystal and thin-film $RuO_2$ samples

Single-crystal $RuO_2$ was grown by chemical vapor transport method. The powder of $RuO_2$ (99.9%, Macklin) was loaded together with $TeCl_4$ in a silica tube. The tube was evacuated and sealed under vacuum. After sealed, the tube was loaded into a two-zone tube furnace with 1393 K (hot zone) and 1293 K (cold zone) for 7 days. High quality thin-film $RuO_2$ was grown on the $TiO_2$(110) substrate in an OMBE chamber [1, 2]. During growth, the substrate temperature was set at 550°C in a distilled ozone background pressure of around $2.0 \times 10^{-6}$ Torr. *In-situ* reflection high-energy electron diffraction (RHEED) was used to monitor the growth process. The crystal structures of $RuO_2$ thin-film samples were characterized via XRD, x-ray reflectivity (XRR) and reciprocal space map (RSM) measurements with Rigaku SmartLab. Magnetic domain images were captured using Photoemission electron microscopy (PEEM) at Beamline 11.0.1 of the Advanced Light Source (ALS). The resistivity was measured in a Quantum Design Physical Properties Measurement System (PPMS).

### ARPES and SARPES measurements

ARPES measurements were performed at BL03U of Shanghai Synchrotron Radiation Facility (SSRF) [3]. Data were measured with a Scienta Omicron DA30 electron analyzer. The energy and angular resolution were set to 10 ~ 20 meV dependent on the photon energy and 0.02 $Å^{-1}$, respectively. Single-crystal samples were cleaved under an ultra-high vacuum of $5.0 \times 10^{-11}$ Torr. While epitaxial thin films were directly transferred to the ARPES chamber under an ultra-high vacuum of $5.0 \times 10^{-10}$ Torr after growth. During measurements, the temperature was kept at T = 14 K, and the pressure was kept better than $5.0 \times 10^{-11}$ Torr. SARPES measurements were performed with a multichannel very-low-energy electron diffraction(VLEED) spin detector attached to a Scienta R3000 hemispherical analyzer using a He I (21.2 eV) light source. The energy and angular resolution were set to 7.2 meV and 0.52°, respectively [4]. For SARPES measurements, epitaxial thin films were transferred to the measurement chamber through an ultra-high vacuum suitcase, the vacuum was kept better than $1.1 \times 10^{-10}$ Torr.

### First-principles calculations

Density functional theory (DFT) calculations were performed within the Vienna *Ab initio* Simulation Package (VASP) [5, 6] to obtain the electronic structures of $RuO_2$. In the calculations of magnetic state, the correlation effects of Ru 4d orbitals were considered by setting U=1.3 eV [7]. To calculate the Fermi surfaces and surface states, the maximally localized Wannier functions [8] were generated by including the d orbitals of Ru atoms and p orbitals of O atoms. The iterative Green's function was applied to get the surface states with a semi-infinite slab [9, 10].

**Supplementary Note 1: Thin films characterization**

Figure S1(a) i shows the RHEED pattern along the [001] direction of the substrate before growth, which serves as a reference to assess the initial surface quality and orientation. The RHEED patterns along the [001] and [1$\bar{1}$0] directions after growth, shown in Figs. S1(a) ii and iii, respectively, exhibit sharp streaks, indicating that the film surface remains smooth and well-ordered post-growth. In addition to the high-resolution XRD measurements shown in Fig. 1, XRR and RSM measurements were conducted to comprehensively characterize the crystal structure, providing complementary information on film thickness, interface quality, and strain. Figure S1(b) presents the XRR data obtained at low incident angles. Genetic algorithms were employed to fit the thickness of three samples, utilizing the pronounced Kiessig fringes observed over a broad angular range, which indicate well-defined interfaces and layer thicknesses. These fits demonstrate that the interfaces between the thin film, substrate, and vacuum are atomically abrupt, and the crystallinity level of the sample along the out-of-plane direction is rather high. Figure S1(c) shows the RSM maps near the 310 and 33$\bar{2}$ Bragg reflections for a 13.5 nm thick $RuO_2$ (110) thin film and the $TiO_2$ substrate, aimed at examining the strain and lattice matching between the film and substrate. The diffuse scattering observed in the thin film indicates partial strain relaxation, suggesting that the film undergoes some degree of strain release as it adapts to the substrate [11]. This partial strain relaxation occurs because $RuO_2$ thin films experience strain constraints induced by the substrates, with mismatches of approximately +1.4%, +2.3%, and -3.1% along the [110], [1$\bar{1}$0] and [001] directions, respectively [12]. Based on the RSM and XRD measurements, we determined the lattice constants of the thin films used for ARPES measurements to be $a$ = 0.45261 nm, $b$ = 0.45107 nm and $c$ = 0.30569 nm, which are crucial for understanding the electronic structure and strain effects.

PEEM, which uses secondary electrons, can image ferromagnetic and antiferromagnetic spin structures through XMCD and XMLD effects. Using circular x-rays at 16° grazing incidence, PEEM is sensitive to both in-plane and out-of-plane magnetization, as shown in Figs. S1(d) i and ii, allowing for comprehensive magnetic domain analysis. Magnetic domain images were captured using PEEM at Beamline 11.0.1 of the ALS. Figure S1(d) iii shows images taken by switching left- and right-circular polarized x-rays, and Figure S1(d) iv shows images taken by switching horizontal- and vertical-linear polarized x-rays, both at a photon energy of 462.1 eV, to differentiate between magnetic domain orientations. All measurements were performed at room temperature with the field view of 28 $\mu$m. Our results showed good thin film morphology of $RuO_2$ and ruled out any magnetic domains with the scale smaller than 28 $\mu$m.

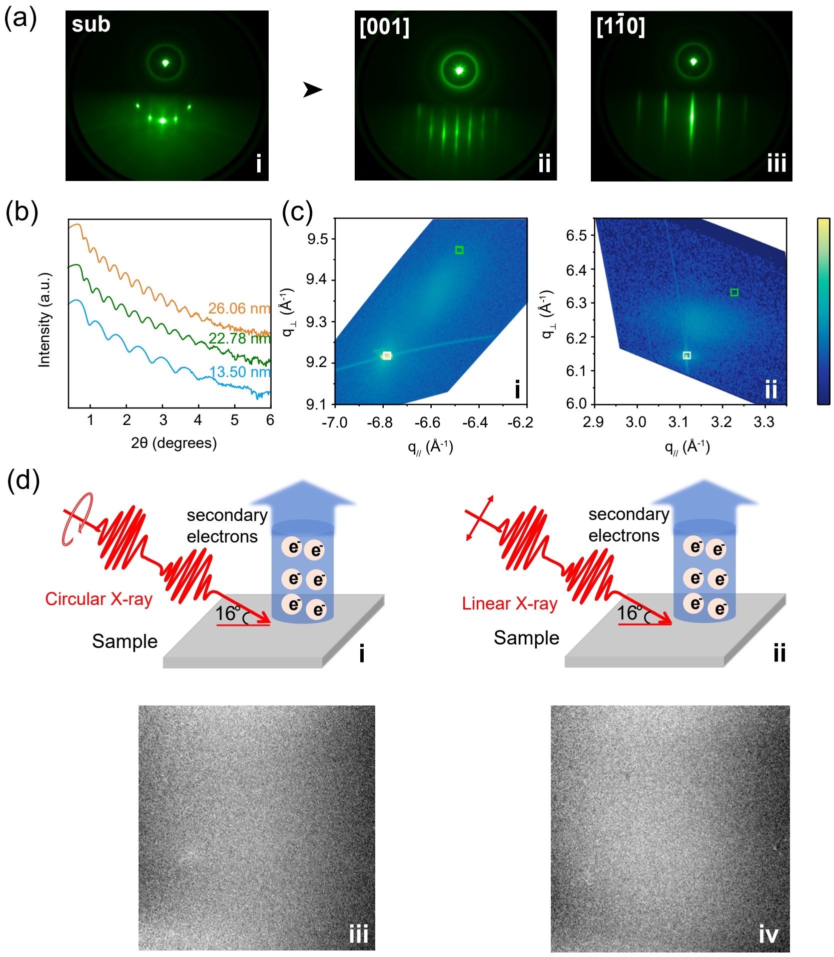


**Fig. S1.** Thin films $RuO_2$ characterization. (a) RHEED patterns of the $TiO_2$(110) substrates and the $RuO_2$(110) thin films along the [001] and [1-10] directions. (b) XRR measurements of thin films with different thicknesses at a low incident angle show clear Kiessig fringes. (c) RSMs for a 13.5 nm thick thin film exhibit partial strain relaxation. The white and green boxes represent the positions of $TiO_2$ substrate and bulk $RuO_2$, respectively. (d) PEEM imaging of $RuO_2$. Schematic drawing of (i) the x-ray magnetic circular dichroism (XMCD) and (ii) x-ray magnetic linear dichroism (XMLD) domain imaging geometry. (iii) XMCD and (iv) XMLD domain images taken at the Ru M edge at room temperature. Both the field view in (iii) and (iv) are 28 $\mu$m.

### Supplementary Note 2: Calculation of band dispersions for the thin film

Figure S2 presents the band dispersions of the thin film. When compared with the band dispersions of single crystals [see Fig. 1(c)], the differences are minimal. The characteristics and trends of the band structures are basically the same for both nonmagnetic and altermagnetic states. In particular, compressive (-3.1%) and tensile (+2.3%) strains are induced along the

[001] and [1$\bar{1}$0] directions, respectively, which do not yet alter the magnetic ground states according to our calculations. While, a slight change in the Fermi level was observed, which corresponds to the global energy shift seen in the ARPES results between the thin films and single crystals, highlighting minor adjustments in their electronic structures.

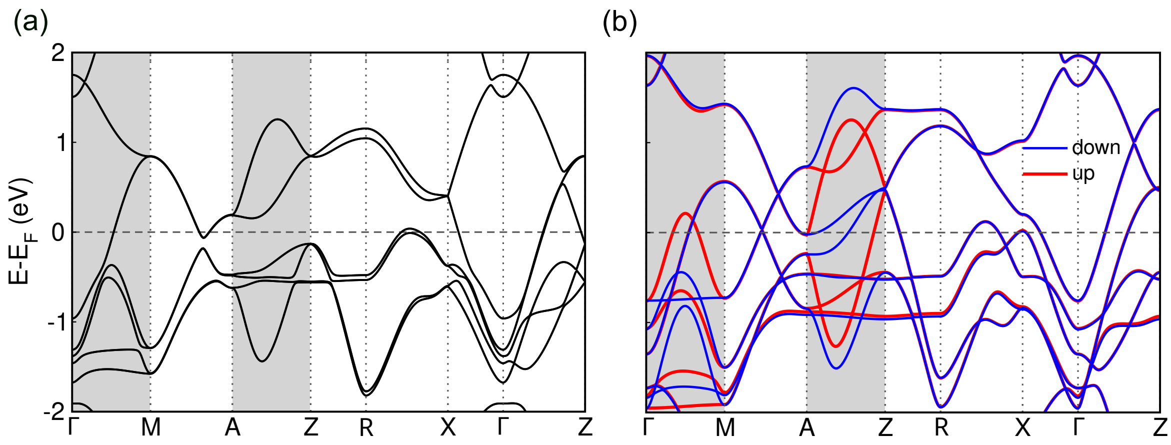


**Fig. S2.** The electronic structures of $RuO_2$ with the lattice constants of thin films. (a) Band dispersions of nonmagnetic state with the consideration of SOC effect. (b) Band dispersions of altermagnetic state without taking consideration of SOC effect but including the correlation effects of Ru 4d orbitals (U=1.3).

**Supplementary Note 3: (110) Fermi surfaces and 3D electronic structures of thin films and single crystals**

Figures S3(a)-(d) display the (110) Fermi surfaces of thin-film samples along $\Gamma$—$M$—$A$—$Z$ and $X$—$R$, alongside their corresponding 3D electronic structures. For comparison, the single-crystal samples are presented in Figs. S3(e)-(h), allowing for a direct assessment of differences and similarities in electronic structure. These two samples exhibit generally consistent low-lying electronic structure features. While, the main difference is that the thin film shows slightly lower quality, evidenced by the disappearance of certain surface states and the presence of only weak flat band surface states.

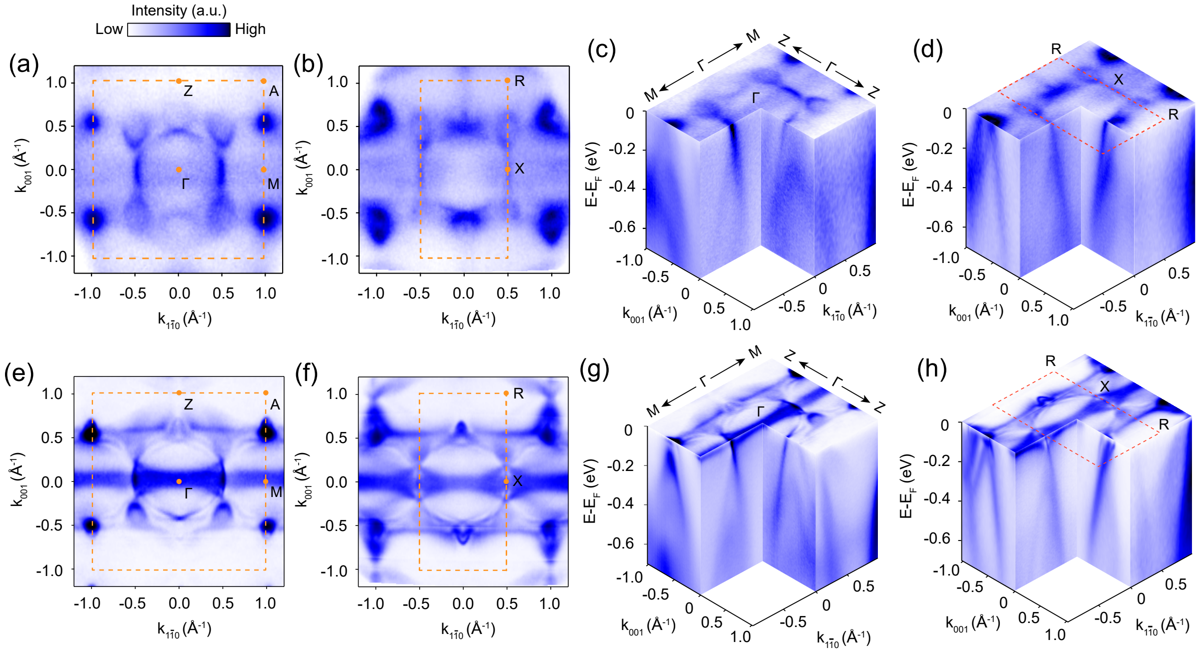


**Fig. S3.** (110) Fermi surfaces and 3D electronic structures. (a)-(d) (110) Fermi surfaces and 3D electronic structures of thin films. (e)-(h) (110) Fermi surfaces and 3D electronic structures of single crystals.

**Supplementary Note 4: Energy resolution exceeds the scale of AM-induced spin splitting**

The energy resolution of our ARPES experiments (Fig. 3, measured with photon energy 124 eV), calibrated using a standard gold sample, is approximately 20 meV, while the SARPES experiment (Fig. 4, measured with photon energy 21.2 eV) achieves a resolution of 7.2 meV [4]. Given these resolutions, we confidently conclude that no spin splitting was detected at an energy scale of 10 meV. As 10 meV approaches the lower bound of typical spin splitting in antiferromagnetic materials, any splitting below this value is more likely to arise from spin-orbit coupling rather than altermagnetism. To further investigate the connection between altermagnetic spin splitting and Ru magnetic moments [13], we present the calculated magnetic band structures along $\Gamma$–$M$ for different Ru magnetic moments in Fig. S4. Even with a reduced magnetic moment of 0.05 $\mu_B$, the predicted spin splitting ( 70 meV) remains well within the detection limit of our experimental resolution. However, none of our measurements

on either single-crystal or thin-film samples revealed such splitting. Therefore, based on the energy resolution of our equipment, we emphasize that no spin splitting greater than 10 meV was observed, which already surpasses the minimum energy scale expected for altermagnetic spin splitting.

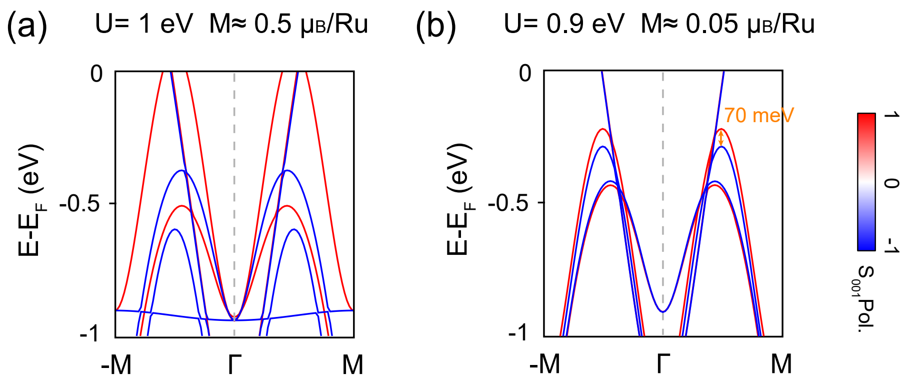


**Fig. S4.** (a) The calculated spin splitting along Γ–$M$ with U = 1 eV and M ≈ 0.5 $\mu_B$/Ru. (b) The calculated spin splitting along Γ–$M$ with U = 0.9 eV and M ≈ 0.05 $\mu_B$/Ru.

**Supplementary Note 5: Energy mismatch between experimental bands and theoretical calculations**

Figure S5 provides confirmation of the "Λ"-shaped bulk states located midway along Γ—$Z$ and near the $Z$ point. These features, identified as hexatruple points, exhibit 6-fold degeneracy when not considering the SOC effect[3, 4], indicating a unique symmetry in the electronic structure [14, 15]. To illustrate this, we selected cut 1 from Figs. S5(a) and S5(b). The corresponding band dispersion and second derivative plots in Fig. S5(d) reveal the Dirac crossing points. Thus, we can identify the remnants of the band crossing, as predicted by DFT calculations, along the Γ—$Z$ direction near the Fermi level (indicated by the yellow arrow in Fig. S5(c), and it should be noted that the SOC effect generates a gap and lifts the 6-fold degeneracy). Our bulk nonmagnetic calculations, consistent with previous studies, do not accurately capture the binding energy position of this feature, which is approximately 0.48 eV lower than predicted [14, 15]. Furthermore, this feature evolves into the Dirac crossing points observed in Figs. S5(e)-(g) along $X$—$R$. Similarly, our calculations in Fig. S5(h) do not predict the correct binding energy position for this feature.

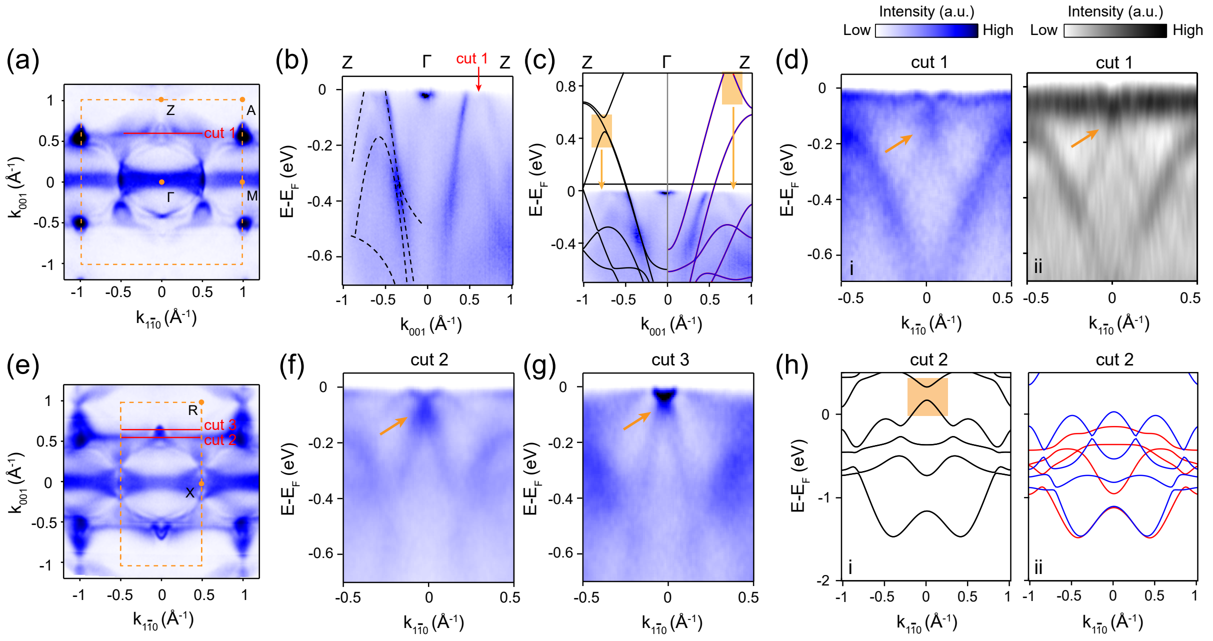

**Fig. S5.** Dirac crossing points. (a) (110) Fermi surface along Γ—*M*—*A*—*Z*. The red solid line marks cut 1. (b) The dispersion of Γ—*Z*. The black dashed lines represent the bands drawn based on the MDCs and second derivative plots. (c) The bands from nonmagnetic (left) and magnetic (right) calculations. The yellow box and arrow indicate that the theoretically predicted bands need to be shifted downward to match the experimental bands. (d) The band dispersion and second derivative plots of cut 1. (e) (110) Fermi surface along *X*—*R*. The red solid lines mark cuts 2 and 3. (f) The band dispersion of cut 2. (g) The band dispersion of cut 3. (h) Cut 2 with nonmagnetic and magnetic calculations.

**Supplementary Note 6: The band dispersion of single crystals and thin films**

We selected Γ—*M*, Γ—*Z*, *M*—*A*, *A*—*Z*, and cuts 1-4 from Fig. S6(a) to display the band dispersion of the single-crystal and the thin-film $RuO_2$ in Figs. S6(b)-(i), in order to provide a comprehensive comparison of their electronic structures. These experimental results are compared with corresponding nonmagnetic and altermagnetic state calculations. To better match the experimental band dispersion, the Fermi level in the nonmagnetic calculations for the single crystals was shifted by 0.06 eV, while in the AM state calculations, it was shifted by 0.18 eV. For thin films, the Fermi level was shifted by 0.18 eV in the nonmagnetic calculations and by 0.29 eV in the AM state calculations. The band dispersion of thin films is generally consistent with that of single crystals, with only some bands shifting upward, as predicted by the thin film calculations. Therefore, the band dispersion of both the single-crystal and thin-film samples aligns more closely with the nonmagnetic calculations, showing no evidence of the band splitting predicted by the AM state calculations. This suggests that the nonmagnetic model is more accurate for describing the electronic structure of $RuO_2$ in both forms.

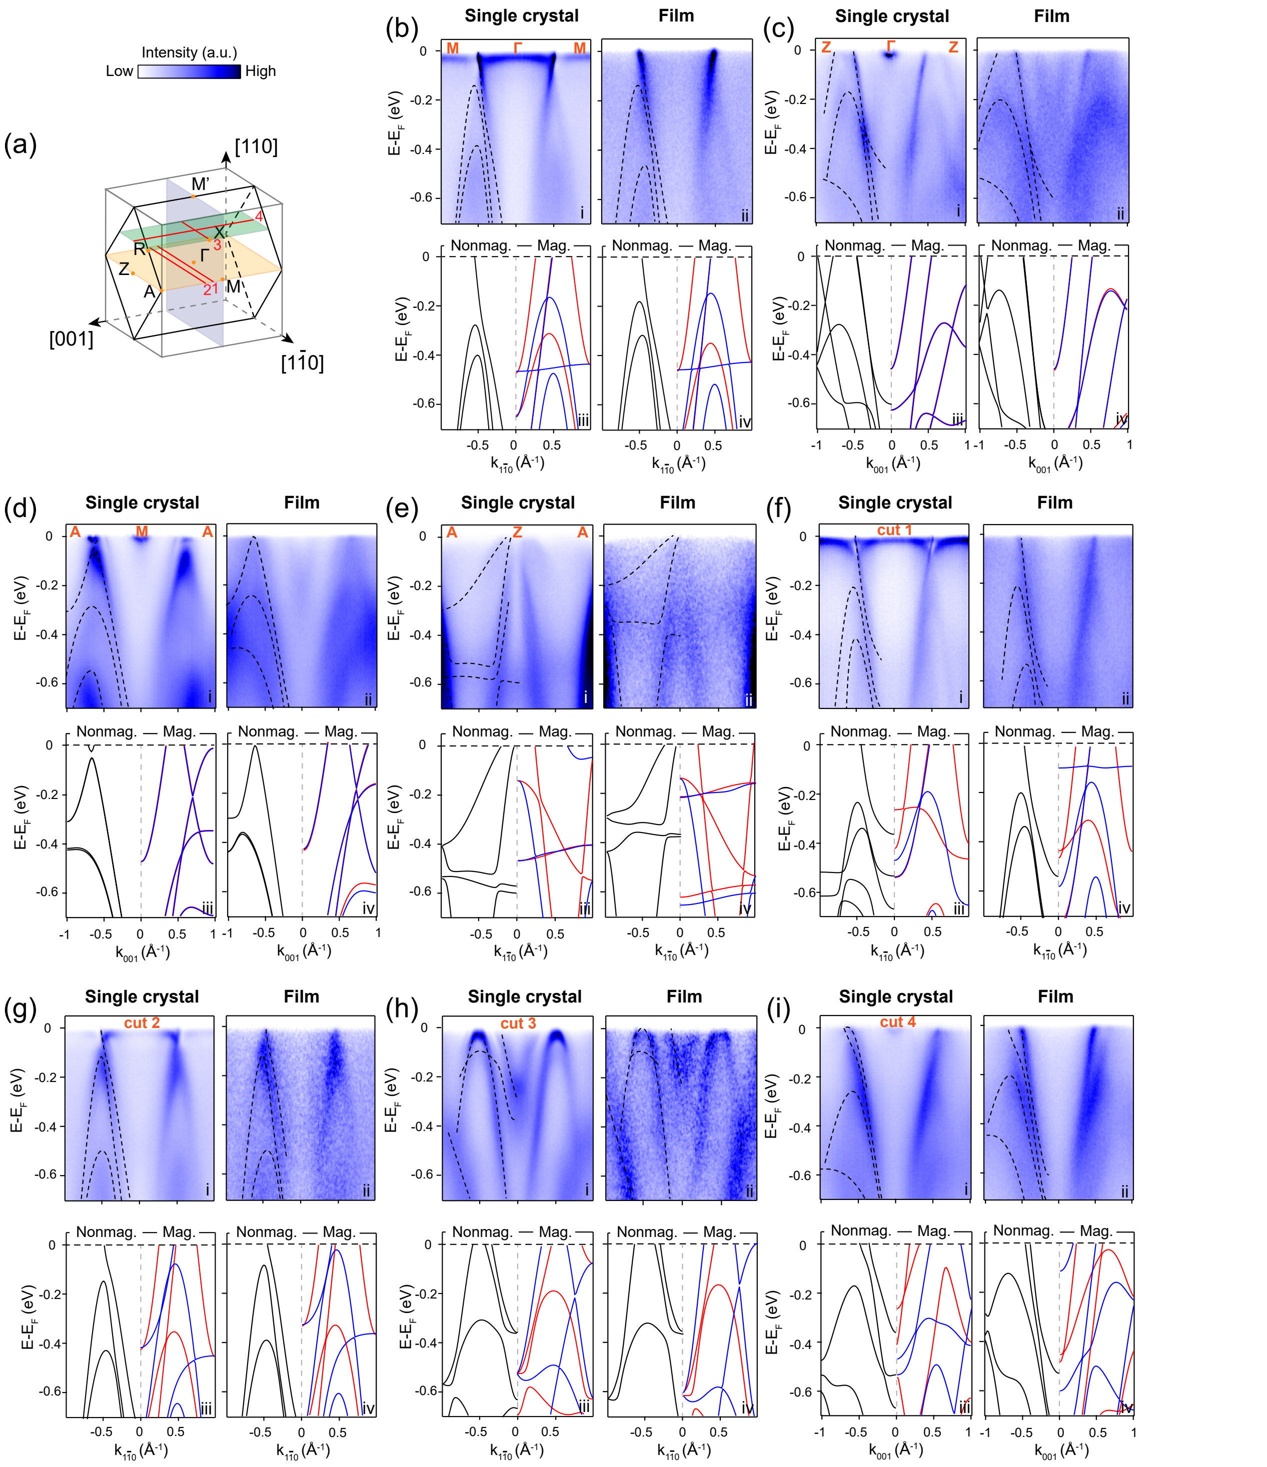


**Fig. S6.** The band dispersion of single crystals and thin films. (a) BZ and the selected four cuts (red solid lines). (b)-(i) The band dispersion of the single-crystal and the thin-film $RuO_2$ compared with nonmagnetic/magnetic calculations. Panels i and iii correspond to the single crystal, while panels ii and iv correspond to the thin film.

**Supplementary Note 7: DFT calculations at photon energy 21.2 eV**

Due to the limitations of the helium lamp, we could not probe the high-symmetry plane $\Gamma$—$M$—$A$—$Z$. Figure S7 shows the nonmagnetic and magnetic calculations corresponding to the photon energy of 21.2 eV. The observed band dispersion matches the nonmagnetic calculations shown in Fig. S7(a). As shown in Fig. S7(b), bands along $\Gamma_1$—$M_1$ and $\Gamma_1$—$M_1$ still exhibit the same spin polarization in this non-high-symmetry plane, in consistency with our SARPES result.

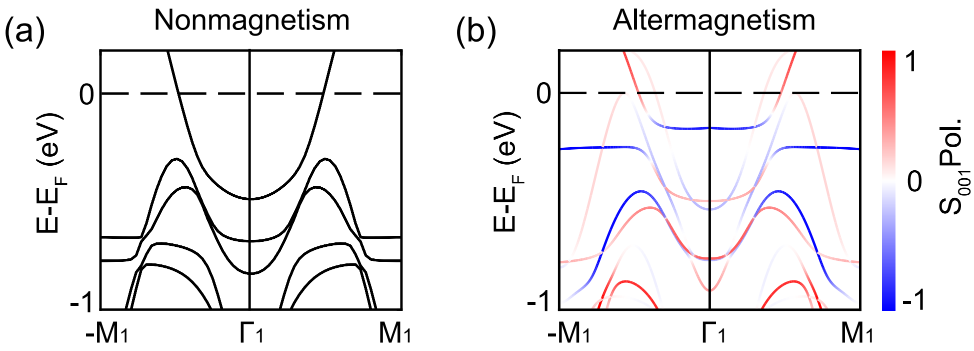


**Fig. S7.** The band structure of $\Gamma_1$—$M_1$ and $\Gamma_1$—$-M_1$ with nonmagnetic and magnetic calculations.

**Supplementary Note 8: SARPES for single crystals**

We present SARPES results on the single-crystal $RuO_2$ samples in Fig. S8. Generally, the spin polarization is consistent with that taken on thin-film samples. We note that the polarization is as high as 0.4.

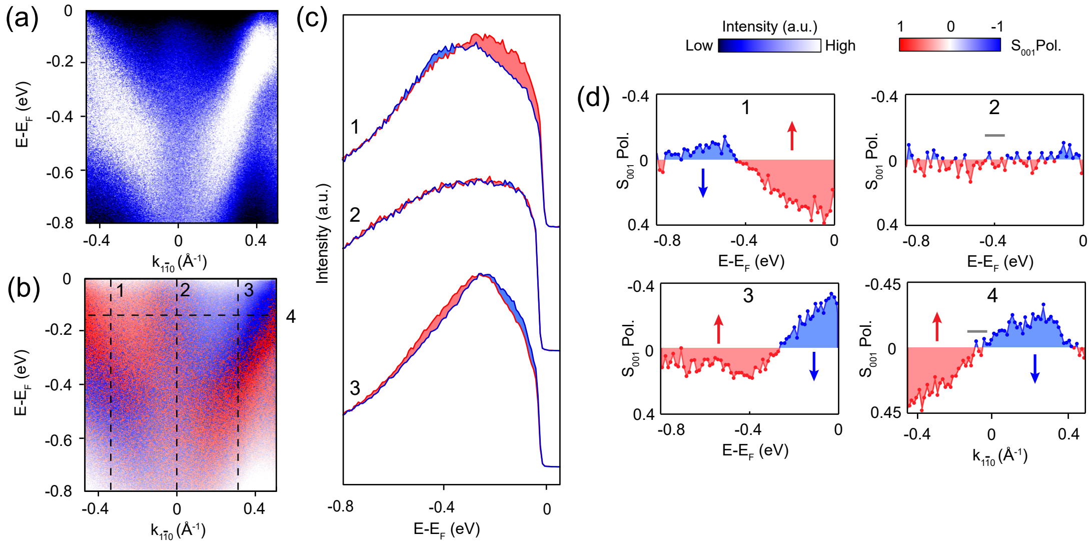


**Fig. S8.** Spin polarization in the single crystal $RuO_2$. (a) Spin-integrated ARPES image. (b) SARPES band dispersion. (c) Spin-resolved EDCs at the three selected momenta. (d) Spin polarization versus binding energy at the three selected momenta. Spin polarization versus momentum at the binding energy of around 0.1 eV.

## Supplementary Note 9: Slab calculations

To further elucidate the observed unusual spin polarization, we performed an 11-layer slab calculation, as depicted in Fig. S9(a), in addition to the Green function calculations shown in Fig. 4(h). Figure S9(b) shows the dependence of the density of states (DOS) and spin polarization on the number of layers in selected region I. The strongly spin-polarized states appear only at the surfaces (first and eleventh layers) and vanish in the intermediate layers, identifying them as surface states. Figure S9(c) indicates that the increase of DOS in the intermediate layers of region II, coupled with an increase in spin polarization, suggests that these states originate from the bulk. The spin polarization observed in layers 4, 5, 7, and 8 corresponds well with our data. These spin-polarized bulk states arise from the bulk continuum reaching the surface boundary. The surface sensitivity of photoelectrons, which allows detection only of the outermost layers, results in Rashba-like states. Figure S9(d) compares the fifth layer of the biased bulk states with the Green function calculations, showing a substantial overlap in the density of states and spin polarization. Thus, both methods provide consistent and corroborative explanations for the observed spin polarization phenomena in the bulk band $\alpha$.

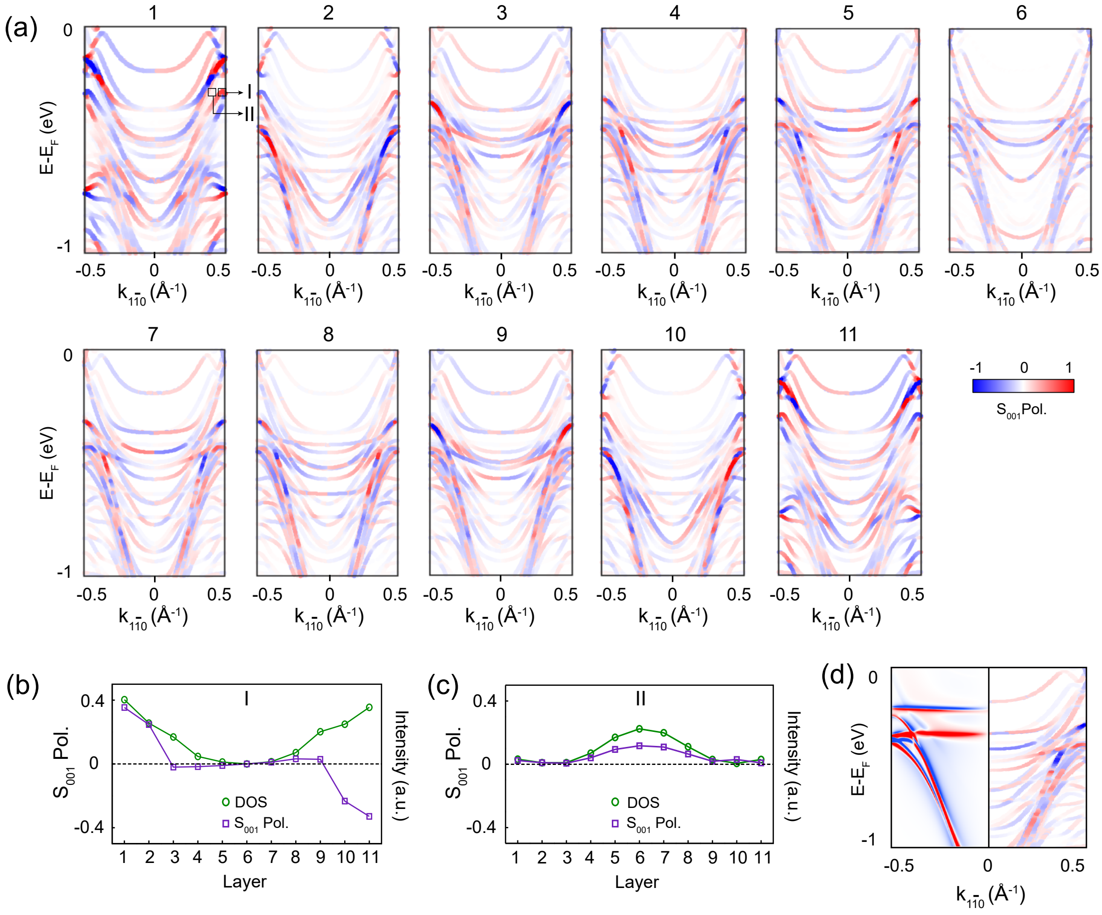


**Fig. S9.** Slab calculations. (a) An 11-layer slab calculation along the Γ—$M$. (b),(c) Layer-dependent average polarization and normalized DOS of regions I and II. (d) Comparison of Green function (left) and slab (right) calculations.

## Supplementary Note 10: Magnetic DFT calculations with oxygen vacancy

Figures. 4(b)-(e) suggest that the bands are highly spin polarized, with an in-plane polarization vector $S_{001}$ antisymmetric about the Γ—$Z$—$M'$ high-symmetry plane. This finding sharply contrasts with the AM ground state prediction for rutile $RuO_2$, in which the bulk band should be fully spin-polarized but symmetric about the plane [as shown in Fig. S10(a)]. Fig. S10(b) lists the bulk space group and the Ru point group for rutile $RuO_2$, along with their respective symmetries. Both ideal and strained $RuO_2$ crystals possess inversion symmetry, thus eliminating the possibility of the Dresselhaus effect and bulk hidden spin polarization observed in some centrosymmetric layered materials [16–18]. While, certain lattice distortions present in the samples, such as local Jahn-Teller distortions, modulation of oxygen vacancies, and distortion of oxygen octahedra, may break local inversion symmetry and give rise to a non-zero electric field [19]. To investigate the unusual spin polarization observed in $RuO_2$, we developed a model based on oxygen vacancies [as shown in Fig. S10(c)]. These vacancies would spontaneously break

the inversion symmetry of the crystal and the centrosymmetry of the Ru site point group, which is expected to result in spin polarization. The resulting band structure, shown in Fig. S10(d), displays opposite spin polarizations on the left and right sides, the oxygen vacancy model is considered only a possible explanation for the observed unusual spin polarization. Additionally, due to the potential influence of oxygen vacancies and substrate-induced strain on the magnetic calculation results, we as well discuss these scenarios in Fig. S10(e) and Fig. S10(f). Our conclusion is that the spin polarization on both sides remains the same, further refuting the presence of magnetism in $RuO_2$. Further theoretical and experimental investigations are needed to determine whether this spin polarization is related to spin-orbit coupling and the spin-polarized currents observed in previous studies.

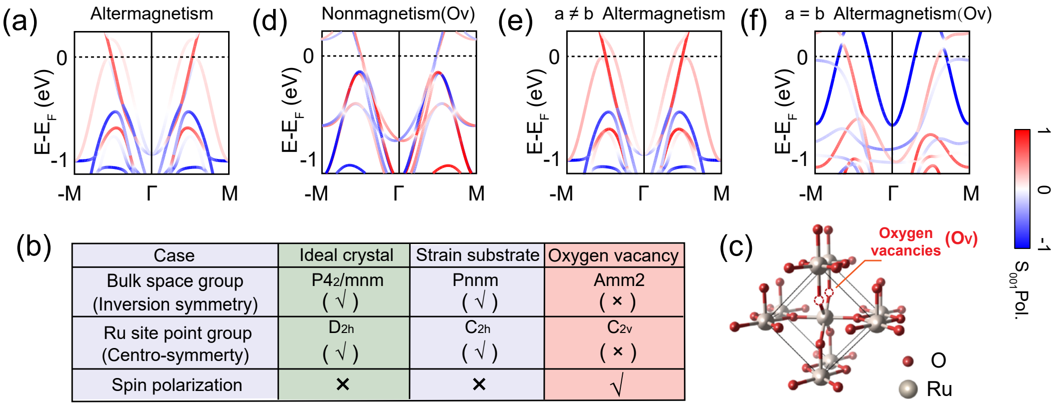


**Fig. S10.** Magnetic DFT calculations with strain/oxygen vacancy. (a) The spin-splitting band structure at Γ—*M* direction predicted by altermagnetic calculations. (b) Summary of the bulk space group, the Ru point group, and spin polarization along with their symmetries in three cases of ideal crystal, strain substrate, and oxygen vacancy. (c) Schematic diagram of $RuO_2$ crystal structure containing 25% oxygen vacancies. (d) The spin polarized band structure along Γ—*M* and Γ—−*M* by nonmagnetic calculations with 25% oxygen vacancies. (e) The spin projection of the altermagnetic case with unequal stress imposed by the substrate. (f) The spin projection of the altermagnetic case with oxygen vacancies.

[1] Lu, X. *et al.* Dimensionality-controlled evolution of charge-transfer energy in digital nickelates superlattices. *Adv. Sci.* **9**, 2105864 (2022).

[2] Ding, J. *et al.* Strain-induced modulation of electronic structure in correlated dirac semimetal Pv-$CaIrO_3$ epitaxial thin films. *J. Vac. Sci. Technol., A* **42**, 032701 (2024).

[3] Yang, Y.-C. *et al.* High-resolution arpes endstation for in situ electronic structure investigations at SSRF. *Nucl. Sci. Technol.* **32**, 31 (2021).

[4] Zha, H. *et al.* Improvement of image-type very-low-energy-electron-diffraction spin polarimeter. *Review of Scientific Instruments* **94** (2023).

[5] Kresse, G. & Furthmüller, J. Efficient iterative schemes for ab initio total-energy calculations using a plane-wave basis set. *Phys. Rev. B* **54**, 11169 (1996).

[6] Dudarev, S. L., Botton, G. A., Savrasov, S. Y., Humphreys, C. & Sutton, A. P. Electron-energy-loss spectra and the structural stability of nickel oxide: An LSDA + U study. *Phys. Rev. B* **57**, 1505 (1998).

[7] Fedchenko, O. *et al.* Observation of time-reversal symmetry breaking in the band structure of altermagnetic $RuO_2$. *Sci. Adv.* **10**, eadj4883 (2024).

[8] Mostofi, A. A. *et al.* wannier90: A tool for obtaining maximally-localised wannier functions. *Comput. Phys. Commun.* **178**, 685–699 (2008).

[9] Wu, Q., Zhang, S., Song, H.-F., Troyer, M. & Soluyanov, A. A. Wanniertools: An open-source software package for novel topological materials. *Comput. Phys. Commun.* **224**, 405–416 (2018).

[10] Sancho, M. L., Sancho, J. L., Sancho, J. L. & Rubio, J. Highly convergent schemes for the calculation of bulk and surface Green functions. *J. Phys. F: Met. Phys.* **15**, 851 (1985).

[11] Ruf, J. P. *et al.* Strain-stabilized superconductivity. *Nat. Commun.* **12**, 59 (2021).

[12] Uchida, M., Nomoto, T., Musashi, M., Arita, R. & Kawasaki, M. Superconductivity in uniquely strained $RuO_2$ films. *Phys. Rev. Lett.* **125**, 147001 (2020).

[13] Smolyanyuk, A., Mazin, I. I., Garcia-Gassull, L. & Valentí, R. Fragility of the magnetic order in the prototypical altermagnet $RuO_2$. *Physical Review B* **109**, 134424 (2024).

[14] Jovic, V. *et al.* Dirac nodal lines and flat-band surface state in the functional oxide $RuO_2$. *Phys. Rev. B* **98**, 241101 (2018).

[15] Jovic, V. *et al.* Momentum for catalysis: how surface reactions shape the $RuO_2$ flat surface state. *ACS Catal.* **11**, 1749–1757 (2021).

[16] Manchon, A., Koo, H. C., Nitta, J., Frolov, S. M. & Duine, R. A. New perspectives for rashba spin–orbit coupling. *Nat. Mater.* **14**, 871–882 (2015).

[17] Feng, Y. *et al.* Rashba-like spin splitting along three momentum directions in trigonal layered ptbi2. *Nat. commun.* **10**, 4765 (2019).

[18] Zhang, X., Liu, Q., Luo, J.-W., Freeman, A. J. & Zunger, A. Hidden spin polarization in inversion-symmetric bulk crystals. *Nat. Phys.*

**10**, 387–393 (2014).

[19] Gotlieb, K. *et al.* Revealing hidden spin-momentum locking in a high-temperature cuprate superconductor. *Science* **362**, 1271–1275 (2018).
